# Supplementary material for: Multimodal Generalized Zero Shot Learning for Gleason Grading using Self-Supervised Learning
Source: arXiv:2111.07646 source file (2021-11-15)
Supplement: Supplementary file 1 [file Suppl_misc.tex]

% this file has the methods section for the MICCAI 2018 paper on active learning based classification

\section{Methods}
\label{sec:met}

\subsection{Intuition behind IDEAL}

Figure~\ref{fig:Histograms} shows two example cases of patients with pleural effusion condition, with high and low levels of uncertainty (accumulated pixel-wise uncertainties via MC Dropout). As we compared the corresponding interpretability saliency (derived from Deep Taylor method \cite{alber2019innvestigate}) and uncertainty maps (shown in Fig.~\ref{fig:Histograms}(b) and Fig.~\ref{fig:Histograms}(d), respectively) and their histograms, Fig.~\ref{fig:Histograms}(c) and \ref{fig:Histograms}(e), we observed that the histograms of high and low informative images are quite distinct, thus verifying the fact that high and low informative images have different values for the most salient regions. Comparing between the high informative image histograms of interpretability saliency and uncertainty maps, we observed that the highest peak of the saliency map histogram (i.e. the ``primary'' peak) has a higher count than the corresponding uncertainty map's histogram ``primary peak''. Additionally, the interpretability saliency map histogram ``secondary peaks'' have lower count than those of the uncertainty map histogram. These point to the fact that, compared to the uncertainty method, the interpretability saliency approach identifies salient regions in a more focused manner. This is beneficial when the goal is to identify the most informative saliency maps for improved classification and segmentation.

% Similarly, we verified how interpretability saliency maps and uncertainty maps vary through the course of training. We selected saliency maps after adding $10\%,20\%,40\%,60\%,90\%$ of training samples. As shown in Figure~\ref{fig:BatchSalMaps}, initially the saliency maps are not well defined since the classifier is not yet trained with sufficient informative samples. However, as more informative samples are being added to the training set, we observe that the saliency maps become more well defined and highlight specific regions of interest. Interestingly, we also observe that saliency maps are sharper and more detailed than uncertainty maps, suggesting an improved description of sample informativeness. The saliency map's informative regions are concentrated and focused on important regions, while the uncertainty maps present dispersed regions. Furthermore at the same percentage of training data, interpretability saliency maps highlight qualitatively better informative regions.

% These seminal observations led us to the hypothesis that saliency maps could be used as a proxy to guide an active sample selection. We investigated this hypothesis by investigating how information from saliency maps could be used to guide sample selection. We studied three different approaches to extract information: starting from a simple histogram feature (stemming from our initial observation), followed by a radiomics-based approach, and finally, an end-to-end deep learning based approach cast as a self-supervised learning problem. 
%
In the following sections we describe the components of the proposed IDEAL approach, including the different investigated information extraction approaches.

\begin{figure*}[t]
\begin{tabular}{c}
\includegraphics[height=6.2cm, width=18cm]{Miccai2020_Latex/Figures/Histogram_Comb1.png} \\
\end{tabular}
\caption{Visualization of saliency maps from different methods. Top row shows a high informative image and bottom row shows a low informative image for pleural effusion condition. (a) original image; (b) saliency map from Deep Taylor method; (c) histograms of saliency  maps for high and low informative images using Deep Taylor; (d) saliency map obtained using Uncertainy; (e) histograms of saliency  maps for high and low informative images using Uncertainty.}
\label{fig:Histograms}
\end{figure*}

\begin{figure*}[htbp]
\begin{tabular}{cccccc}
\includegraphics[height=2.2cm, width=2.5cm]{Miccai2020_Latex/Figures/Batch_Image5_Original.png} &
\includegraphics[height=2.2cm, width=2.5cm]{Miccai2020_Latex/Figures/Batch_Image5_10.png} &
\includegraphics[height=2.2cm, width=2.5cm]{Miccai2020_Latex/Figures/Batch_Image5_20.png} &
\includegraphics[height=2.2cm, width=2.5cm]{Miccai2020_Latex/Figures/Batch_Image5_40.png} &
\includegraphics[height=2.2cm, width=2.5cm]{Miccai2020_Latex/Figures/Batch_Image5_60.png} &
\includegraphics[height=2.2cm, width=2.5cm]{Miccai2020_Latex/Figures/Batch_Image5_90.png} \\
%------------
% &
% \includegraphics[height=2.2cm, width=2.5cm]{Miccai2020_Latex/Figures/Batch_Image5_10_Unc.jpg} &
% \includegraphics[height=2.2cm, width=2.5cm]{Miccai2020_Latex/Figures/Batch_Image5_20_Unc.jpg} &
% %
% \includegraphics[height=2.2cm, width=2.5cm]{Miccai2020_Latex/Figures/Batch_Image5_40_Unc.jpg} &
% \includegraphics[height=2.2cm, width=2.5cm]{Miccai2020_Latex/Figures/Batch_Image5_60_Unc.jpg} &
% \includegraphics[height=2.2cm, width=2.5cm]{Miccai2020_Latex/Figures/Batch_Image5_90_Unc.jpg} \\
%------------
&
\includegraphics[height=2.2cm, width=2.5cm]{Miccai2020_Latex/Figures/Unc_10.png} &
\includegraphics[height=2.2cm, width=2.5cm]{Miccai2020_Latex/Figures/Unc_20.png} &
\includegraphics[height=2.2cm, width=2.5cm]{Miccai2020_Latex/Figures/Unc_40.png} &
\includegraphics[height=2.2cm, width=2.5cm]{Miccai2020_Latex/Figures/Unc_60.png} &
\includegraphics[height=2.2cm, width=2.5cm]{Miccai2020_Latex/Figures/Unc_90.png} \\
(a) & (b) & (c) & (d) & (e) & (f)\\
\end{tabular}
\caption{Uncertainty maps (top row), and interpretability saliency maps (bottom row) for a given sample input image at different training data levels. (a) Original image (b) $10\%$ of informative samples (c) $20\%$ of informative samples; (d) $40\%$ of informative samples; (e) $60\%$ of informative samples; (f) $90\%$ of informative samples. }
\label{fig:BatchSalMaps}
\end{figure*}

\subsection{Main components of IDEAL}

Figure~\ref{fig:IDEALPipeline} depicts a general pipeline of the proposed IDEAL approach. Given unlabeled testing samples (i.e. sample pool), and an associated deep learning classification model (e.g. DenseNet) trained iteratively during active learning, an interpretability saliency map generator is used to produce saliency maps, from which a sample informativeness score (IDEAL Scoring) is calculated to rank pool samples by their informativeness. The IDEAL scoring can be produced in different ways, depending on how the information from the saliency maps is distilled to produce a ranking score for each pool sample. In this study we investigated three different ways of extracting information and scoring samples, which are presented in order of complexity: (i) From our original observation, a single feature extracted from the histogram of saliency maps (Fig.~\ref{fig:Histograms}(c)) is used to derive the IDEAL scoring, (ii) Multivariable radiomics features are extracted and combined into single IDEAL scores, and (iii) Our proposed novel Deep features extracted and used within a self-supervised approach to score informative samples.

In the following we describe each component in detail and in relation to the clinical problem of automating lung disease classification and histopathology segmentation, as well as baseline methods used to benchmark the proposed IDEAL approach.

\begin{figure*}[t]
\includegraphics[height=4.2cm,width=18.0cm]{Miccai2020_Latex/Figures/IDEALPipeline.png} 
\caption{Proposed IDEAL approach. Given testing samples (i.e. pool samples) and a trained classifier, interpretability saliency maps are generated for each testing sample, and an \textit{IDEAL} score is generated from the saliency maps to characterize sample informativeness. Top-ranked samples are then prioritized for label query and for the next active learning training cycle.}
\label{fig:IDEALPipeline}
\end{figure*}

\subsection{Classification model}

The classification model is not per se a component of the IDEAL approach but rather an input its calculations are based on. We present it here to facilitate the presentations and descriptions of the data workflow, as presented in Fig.~\ref{fig:IDEALPipeline}. Any robust classification model can be used as the approach is not restricted to particular architectures. For lung disease classification from X-ray images, we experimented with $3$ different models namely, DenseNet-121 \cite{CheXNet},ResNet-50 \cite{ResNet} and VGG16 \cite{VGG}, and found the DenseNet-121 architecture to perform the best. We denote as $M$, the DenseNet-121 model, and point the reader to section \ref{sec:impldetails}, for further implementation details of the trained model. \snm{For the histopathology image segmentation task we used a DenseNet-121 classifier of the histopathology images (benign vs. malign), as a proxy of informativeness for the main task of image segmentation. This was motivated by multi-task learning where tasks are typically intertwined, and the availability of interpretability approaches for classification tasks. As shown in the results section, we show that this approach is effective in the segmentation task as well.} 

\subsection{Interpretability Saliency Map Generator}

Image-specific saliency maps operate under the the basic principle of highlighting areas of an image that drive the prediction of a model. The importance of these areas can be obtained by investigating the flow of the gradients of a DL model calculated from the model’s output to the input image, or by analyzing the effect of a pixel (or region) to the output when that pixel (or region) is perturbed. This type of visualization facilitates interpretability of a model but also serves as a confirmatory tool to check that machine-based decisions align with common domain knowledge \cite{Reyes2020}. As mentioned, differently from previous works in interpretability, we aim here to employ saliency maps to perform active sample selection. 
To generate interpretability saliency maps we use the iNNvestigate library \cite{alber2019innvestigate} \footnote{https://github.com/albermax/innvestigate}, which implements several known interpretability approaches. We employ Deep Taylor, a known interpretability approach to generate saliency maps, due to its ability to highlight informative regions while yielding minimal importance to other regions. Deep Taylor operates similarly as other interpretability approaches by decomposing back-propagation gradients, of the studied model, into layer-wise relevance maps of individual cell activations, as a function of a queried input sample and class label (e.g. disease class)\cite{montavon2017explaining}.

\subsection{IDEAL Sample Informativeness Score}
In this section we formalize the definition of the IDEAL sample scoring. Given a test image $I \in R^{m \times n}$, a prediction model $M$ being updated via active learning, and the corresponding saliency map $S(I,M) \in R^{m \times n}$, we map the saliency map $S(I,M)$ into a sample informativeness score, termed IDEAL score as:

% \begin{equation}
% IDEAL_{score}:S(I,M)\in R^{m \times n} \rightarrow f \in R.
% \label{eq:IDEALScore}
% \end{equation}

\begin{equation}
IDEAL_{score}:f(S(I,M))\in R^{m \times n} \rightarrow R.
\label{eq:IDEALScore}
\end{equation}

The function $f$ can have different forms, depending on the way the information is extracted from the saliency map and converted into an informative sample score. We present results investigating three different approaches, described in further detail below.

%\begin{enumerate}
%    \item \textbf{Single Hand-crafted Feature - Kurtosis}: From the seminal observations we designed a simple single feature based on the \textit{kurtosis} operator, describing the changes visible in the histogram of high and low uncertainty samples (Fig.~\ref{fig:Histograms}(c))  
    %\item \textbf{Multivariate Radiomics Features}: We explored %radiomics-based features, which describe different types of information from the saliency maps. Radiomics features are then combined  
    %\item \textbf{Deep Saliency Features}: A feature extractor network is used to extract features in an unsupervised way, followed by a self-supervised based ordinal clustering of informative samples.
%\end{enumerate}

The IDEAL scores obtained for the set of testing samples are sorted in decreasing order and the top-n ranked samples are chosen for expert label querying and added to the next active learning cycle. The complete IDEAL process is summarized in Algorithm~\ref{alg1}. In Algorithm~\ref{alg1} the model $M_0$ can be  a pretrained network or, as in our experiments, trained with a small part of the training dataset (e.g. 10\% of training). 

\begin{algorithm}
\caption{Interpretability-Driven Sample Selection - IDEAL}\label{alg1}
\begin{algorithmic}[1]
\Require Pretrained model $M_0$, \textit{Saliency map operator} $S(\dot)$, $\mathbb{I}_{validation}$, $AUC_{target}$ 
\State $M \leftarrow M_0$ 
\Repeat
\State $\mathbb{I}_{in} \leftarrow \{I_{in}\}$ \Comment{define set of input testing images}
\State $\mathbb{S}_{in} \leftarrow \{S(\mathbb{I}_{in},M)\}$ \Comment{saliency maps given input set and current model}
\State $\{ scores \}_{in} \leftarrow IDEAL_{score}(\mathbb{S}_{in}) $ \Comment{calculate informativeness scores}
\State $ \mathbb{I}_{sort} \leftarrow sort(\mathbb{I}_{in},\{scores\}_{in})$ \Comment{sort $\mathbb{I}_{in}$ in decreasing order by scores}
\State $\mathbb{I}_{train} \leftarrow \mathbb{I}_{sort}\{i=1,...,top\_n\}$ \label{alg1:topn} \Comment{select top-n ranked samples}
\State $\mathbb{L}_{train} \leftarrow expert\_query(\mathbb{I}_{train})$ \Comment{label querying of selected samples}
\State $M_{new} \leftarrow train(M,\mathbb{I}_{train},\mathbb{L}_{train})$ \Comment{train new model}
\Until{$AUC(M_{new},\mathbb{I}_{validation}) \geq AUC_{target}$} \Comment{Repeat until target AUC is attained}\\
\Return $M_{new}$
\end{algorithmic}
\end{algorithm}

We now describe in detail each of the three studied feature extractor approaches:

%%%%% Single Hand-crafted Feature - Kurtosis %%%%
%%%%%%%%%%%%%%%%%%%%%%%%%%%%%%%%%
\vspace{5pt}
\subsubsection{\textbf{Single Hand-crafted Feature - Kurtosis}}
This first approach is motivated by the observation made from the histograms between high and low uncertainty samples, Figure~\ref{fig:Histograms}. As operator $f$ in Equation~\ref{eq:IDEALScore}, we defined $f=k(H(S(I)))$, with  $H$ and $k$ corresponding to the histogram and kurtosis operators, respectively. Consequently, and based on our observations, informative samples are associated to larger kurtosis values and sorted accordingly to select informative ones. In the results section, this approach is referred to as \textit{Kurtosis}.

%%%%% Multivariate Radiomics Features %%%%
%%%%%%%%%%%%%%%%%%%%%%%%%%%%%%%%%%%%%%%%%%
\vspace{5pt}
\subsubsection{\textbf{Multivariate Radiomics Features}}
As second approach, we used the PyRadiomics package \cite{Pyrad} to extract different radiomics features from the saliency maps. Owing to the large number of potential features we employ a feature selection strategy. \snm{ PyRadiomics has 8 feature categories. We trained random forest (RF) classifiers to predict the image's disease label using each feature category. Based on the in-built information gain of the RF model, we identified the $3$ best performing categories as: ``First Order Statistics'' ($19$ features), ``Gray Level Co-occurrence Matrix (GLCM)'' (24 features), and ``Shape Based (2D)'' ($10$ features). The final features for each category is identified by performing an exhaustive search over all possible feature combinations and using it to predict disease labels with a RF classifier. The final features are summarized in Table~\ref{tab:features}.   } 

% consisting of the following steps:

% \begin{enumerate}
%     \item Step 1: PyRadiomics has 8 feature categories. We trained random forest (RF) classifiers using each category, and based on the in-built information gain of the RF model, we identified the $3$ best performing categories as: ``First Order Statistics'' ($19$ features), ``Gray Level Co-occurence Matrix (GLCM)'' (24 features), and ``Shape Based (2D)'' ($10$ features).
    
%     \item Step 2: For each selected category, we train RFs on every possible feature combination and identified the most informative features. For example, for the category `First Order Statistics'' there are $2^{19}-1=524,287$ feature combinations, out of which the best performing feature set was, in order of decreasing importance, `Kurtosis', `Skewness', `Entropy' and `Total Energy'. Similarly, for GLCM, out of $16,777,215$ combinations we identified the best performing feature set as `Sum Entropy',`Inverse Difference Normalized',`Difference Entropy', and `Maximal Correlation Coefficient'. For the category ``Shape 2D'' we identified, out of $1023$ combinations, `Sphericity', `Spherical Disproportion', and `Elongation' as the best performing feature set.
% \end{enumerate}

In order to combine extracted selected radiomics features for ranking, \snm{we rank different metrics based on the Borda count, which has been used before for ranking informative samples \cite{OzdemirDLMIA2018}. With Borda count samples are ranked for
each metric, and samples are selected based on the best combined rank as:
\begin{equation}
    i^{*}=\arg \min_i \left(\sum_{m_k} f_{rank} m_k(I_i) \right)
\end{equation}
where $m_k$ denotes the $k^{th}$ pyradiomic feature calculated on image $I_i$.
}
In the results section, this approach is referred to as \textit{PyRad\_category}, with \textit{category} being one of the following \textit{\{1st-order, GLCM, 2DShape\}}.

\begin{table}[!htbp]
 \begin{center}
 \caption{Description of selected Pyradiomics and Deep Saliency Features.}
\begin{tabular}{|l|l|}
\hline 
{\textbf{Feature Type}} & {\textbf{Comments}} \\ \hline
{Kurtosis} & {Obtained from histogram of the intensity distribution} \\ \hline
{Radiomics-} & {Initial $19$ features. Exhaustive search on $2^{19}-1$} \\ 
{First Order} & {combinations. $4$ best features - `Kurtosis',  `Skewness',} \\
 {} & {`Entropy'  and  `Total  Energy'.} \\ \hline
 {Radiomics-} & {Initial $24$ features. Exhaustive search on $2^{24}-1$ } \\ 
{GLCM} & {combinations. $4$ best features -`Sum Entropy',`Inverse  } \\
 {} & {Difference  Normalized',`Difference  Entropy' and } \\ 
 {} & { ‘Maximal  Correlation  Coefficient’.} \\ \hline
  {Radiomics-} & {Initial $10$ features. Exhaustive search on $2^{10}-1$ } \\ 
{Shape} & {combinations. $3$ best features -`Sphericity’, ‘Spherical  } \\ 
{} & {Disproportion’,  and‘Elongation’} \\ \hline
  {Deep Saliency} & { Ordinal Clustering of latent feature vector} \\ 
{Features} & { followed by Self-Supervised step. Details in text. } \\ \hline
\end{tabular}
\label{tab:features}
\end{center}
\end{table}

%%%%% Deep Saliency Features %%%%
%%%%%%%%%%%%%%%%%%%%%%%%%%%%%%%%%
\vspace{5pt}
\subsubsection{\textbf{Deep Saliency Features: Ordinal Clustering And Self Supervised Learning For Informative Sample Selection}}
\label{met:ordinal}

In this section we present the third and more advanced approach. We propose a novel approach that uses deep features extracted from an autoencoder and self supervised learning based ordinal clustering of informative samples.

The goal in self-supervised learning is to identify a suitable self supervision task (or pretext task) that provides additional knowledge (in the form of network weights) to successfully train a model to solve the main task. Some common pretext tasks include for example, estimating relative position of patches \cite{Doersch,Noroozi}, local context \cite{Pathak}, and colour \cite{ZhangECCV2016}. Additionally, exemplar learning has been proposed as a self-supervised learning strategy \cite{Dosovitskiy} where the task is to classify each data instance into a unique class. 

Given a set of candidate pool samples, saliency maps are generated and, as first step, an auto encoder is trained to reconstruct them. %\snm{As shown in Figure~\ref{fig:SSOrdinal} the encoder stage has 3 layers of $256,128,64$ neurons. The output is a $32$ dimensional latent feature vector which is fed to the decoding stage. The output is supposed to reconstruct the original input using the mean square error loss.}
The output of the encoding stage is a $l-$dimensional latent feature vector representation (referred to as \textit{Deep Saliency Features}), which is used as input for the next stage of ranking them. In order to discriminate informative samples from Deep Saliency Features, and in the absence of information to distill which Deep Saliency Features are associated to sample informativeness, we cast the problem as a self supervised learning approach to assign informativeness labels to saliency maps. Figure~\ref{fig:SSOrdinal} depicts the proposed self supervised learning approach, which is also explained in Algorithm~\ref{alg2}. It consists of the following steps:

\begin{enumerate}
    \item Extracted latent feature vector representations are clustered using an ordinal cluster approach into $K(=10)$ clusters. %\snm{In our experiments we chose $K=10$ to provide enough granularity in the number of samples per cluster. A high number of clusters can result in no samples per cluster, while too few clusters can lead to a lack of differentiation among samples.}
     %\begin{enumerate}
    %\item In practice we chose $K=10$ clusters. 
    %\item A batch size of $32$ gives an average of $3$ samples per cluster -- a %reasonable number to determine informativeness. 
    %\item Too high $K$ results in no samples for certain clusters while too low $K$ %loses granularity of informativeness. % to have a reasonably fine grained %informative scale for sample selection, although this number can vary depending upon %batch size.
    %\end{enumerate}
    
    \item Identify most representative sample of each cluster via measuring the closest  sample to its centroid using L2 distance between extracted latent feature vectors.
    
    \item Query labels of the most representative sample per cluster (e.g. $K=10$ queries)
    
    \item Add the corresponding original image to the training set, and determine the change in AUC values ($\Delta AUC$) for a fixed validation set (independent of the training set). Rank samples according to decreasing $\Delta AUC$.
    
    \item Identify cluster whose representative image yields maximum positive $\Delta$AUC on validation set.
    \begin{enumerate}
        \item Select this cluster as most informative
        \item Label each cluster as $[1,\cdots,K]$ where $1$ is most informative cluster and $K$ denotes least informative cluster. 
        \item Ranking and queried labels for each representative sample are propagated to all samples within each cluster. 
        % \item Thus pool samples are implicitly labelled and ranked through their representatives.
    \end{enumerate}
    
    \item Use labelled samples from the previous step, and their corresponding deep saliency features to train a random forest classifier. \snm{In order to efficiently train the random forest classifier as new samples are selected, we use online random forests \cite{onlineRF}, which performs incremental training of the RF using the previously trained RF as a starting point. The saliency map is classified into one out of $K$ possible levels of informativeness. Use $RF_{final}$ (Algorithm~\ref{alg2}) to rank new (test) samples based on informativeness. }
    % \begin{enumerate}
    % \item Classify saliency map into one . 
    % \end{enumerate}
    
\end{enumerate}

\snm{The choice of $K=10$ was to strike a balance between level of granularity and avoid clusters with too few or no samples. If $K$ is too high then we have to increase the batch size (from 32 to higher) to ensure sufficient samples in each cluster for accurately determining a representative vector. However, increased batch size leads to higher computation cost and poses challenges during training. If $K$ is too low then we lose granularity of informativeness rankings. For example, if $K=5$ then samples with different levels of informativeness will be in one cluster and make it difficult to train a reliable classifier to predict informativeness. Thus $K=10$ gives the best tradeoff between these two considerations. 
}

\begin{algorithm}

\caption{Self Supervised Deep Features - Training Stage  }
\label{alg2}
\begin{algorithmic}[1]

\Require \snm{Random forest $RF_0$, Set of Deep Saliency feature vectors $F$, \textit{Ordinal Clustering operator} $C(\dot)$, number of clusters $K$, $\mathbb{I}_{validation}$, $\mathbb{I}_{train}$}
\State \snm{$RF \leftarrow RF_1 , n=1$ }
\Repeat
\State \snm{$\mathbb{F}_{n} \leftarrow \{F_{n}\}$ \Comment{Feature vectors for iteration $n$}
\State $\mathbb{C}_{n} \leftarrow \{C(\mathbb{F}_{n})\}$ \Comment{clustering output given input set and clustering operator}}
\State \snm{Identify representative samples of each cluster $\mathbb{F}_{rep}$ \Comment{sample closest to each cluster's centroid}}
\State \snm{Identify corresponding original images $\mathbb{I}_{rep}$
\State Query  label  of  most  representative  sample  per  cluster \Comment{For all K clusters}}
\State \snm{$\mathbb{L}_{rep} \leftarrow expert\_query(\mathbb{I}_{rep})$ \Comment{label querying of representative samples}}
%
% \State \snm{$\mathbb{I}_{train} \leftarrow \mathbb{I}_{rep}$, $\mathbb{L}_{train} \leftarrow \mathbb{L}_{qrep}$ \label{alg2:topn} \Comment{add queried images to training set}}
% \State $\mathbb{L}_{train} \leftarrow expert\_query(\mathbb{I}_{train})$ \Comment{label querying of selected samples}
\State \snm{$RF_{n} \leftarrow train(RF_{n-1},\mathbb{I}_{rep},\mathbb{L}_{rep})$ \Comment{update pre-trained model using online RF}
\State Identify cluster $k$ with highest $+\Delta$AUC
\State Label  each  cluster $[1,\cdots,K]$ \Comment{$1$ is  most informative cluster and $K$ is least informative}}
\State \snm{$\mathbb{I}_{train}=\mathbb{I}_{train} \setminus \mathbb{I}_{rep}$  \Comment{Update training set}
\State $n \leftarrow n+1$ \Comment{Go to next iteration}
\Until{$\mathbb{I}_{train}=\emptyset$} \Comment{Repeat until all training samples are used }}\\
\Return \snm{$RF_{final}$ \Comment{Random forest classifier that ranks samples based on informativeness}}
\end{algorithmic}
\end{algorithm}

The proposed ordinal clustering and self supervised learning approach for informative sample selection leverages feature extraction information using modern deep learning technologies. This comes at the cost of a minimal label expert querying of representative samples (i.e. number of cluster $K)$, which based on our experience and the results obtained, yields a good trade-off for clinical utilization. 

In the results section this approach is referred to as \textit{Deep Features}.
In the next section we present results obtained with the proposed and baseline approaches, along with several ablation experiments aiming at leveraging further insights and confirmatory evidence on the benefits of the proposed IDEAL approach.

\begin{figure*}[t]
\begin{tabular}{c}
\includegraphics[height=7.4cm,width=16.0cm]{Miccai2020_Latex/Figures/Workflow1.png} \\
\end{tabular}
\caption{Workflow for Ordinal Clustering and Self Supervised learning for informative sample selection. Deep features extracted from an autoencoder are used for ordinal clustering samples into to $K (e.g. K=10)$ clusters. Representative images from each cluster (i.e. samples closest to each cluster's centroid) are queried for labels and added to the training set. Changes in AUC values on a validation set are determined after updating the classification model. Based on $\Delta$AUC of each cluster's representative image, the $K$ clusters are assigned different levels of informativeness in a self supervised manner. Labels and ranking of representative samples are propagated to samples within each cluster, and random forest is trained on to learn to classify each saliency map into each of $K$-level informative levels. }
\label{fig:SSOrdinal}
\end{figure*}

\section{Baseline Methods For Comparison}
\label{sec:baselines}
In this section we describe the baseline methods used for comparison purposes.

\subsection{Standard Active Learning}
As first baseline we considered a standard active learning framework where no sample selection is considered. In this setup, given a set of testing samples, a subset of samples are randomly chosen for label querying and active learning training. It is worth noting, that in clinical practice the number of samples reflects the amount of user interaction needed to incorporate new samples into the next cycle of active learning, and hence it needs to be kept as low as possible. In the results section we refer to this approach as \textit{Random}. %In the results section we further analyze this aspect of required user interaction and learning performance.

\subsection{Uncertainty-driven sample selection}

This corresponds to our second baseline. As proposed in \cite{MahapatraMICCAI2018, BozorgtabarCVIU2019}, uncertainty estimation can be used as a metric of sample informativeness for active learning. %Several approaches have been proposed to estimate uncertainty on input samples. We adopted the approach presented in \cite{BDNN}, as also originally proposed by \cite{MahapatraMICCAI2018, BozorgtabarCVIU2019} to assess sample informativeness in an active learning setup. G
 Given the deep learning model $M$ used for disease classification, mapping an input image $I$, to a unary output $\widehat{y}\in R$, the predictive uncertainty for pixel $y$ is approximated using:
\begin{equation}
Var(y)\approx \frac{1}{T} \sum_{t=1}^{T} \widehat{y}_t^{2} - \left(\frac{1}{T} \sum_{t=1}^{T} \widehat{y}_t \right)^{2} + \frac{1}{T} \sum_{t=1}^{T} \widehat{\sigma}_t^{2}
\label{eqn:Uncert}
\end{equation}
$\widehat{\sigma}^{2}_t$ is the model's output for the predicted variance for pixel $y_t$, and ${\widehat{y}_t,\widehat{\sigma}^{2}_t}^{T}_{t=1}$ being a set of $T$ sampled outputs.

Similarly as for the other compared approaches, the obtained uncertainty estimates are sorted from high to low uncertainty, and the \textit{top-n} samples are chosen for label querying, and added to the next active learning cycle.  In the results section we refer to this approach as \textit{Uncertainty}.

\subsection{Implementation details}\label{sec:impldetails}

Our method was implemented in TensorFlow. We trained DenseNet-121 \cite{DenseNet} on \snm{NIH
ChestXray14} dataset \cite{NIHXray}, and for the histopathology datasets. We used Adam \cite{Adam} with $\beta_1=0.93$, $\beta_2 = 0.999$, batch normalization, binary cross entropy loss, learning rate $1e-4$, $10^{5}$ update iterations and early stopping based on the validation accuracy. %The network was fine-tuned using the validation set (see section  \ref{sec:data}). 
The architecture and trained parameters were kept constant across compared approaches. Training and test was performed on a NVIDIA Titan X GPU having $12$ GB RAM.
Images are fed into the network with size $320 \times 320$ pixels. %We use the Adam optimizer with default $\beta$-parameters of $\beta_1 = 0.9$, $\beta_2 = 0.999$ and learning rate $1 × 10^{−4}$ which is fixed for the duration of the training.

We employed 4-fold data augmentation  (i.e. each sample augmented 4 times) using simple random  combinations of rotations ($[-25,25]^{\circ}$), translations ($[-10,10]$ pixels in horizontal and vertical directions), and isotropic scaling ($[0.95-1.05]$ scaling factors).
For generation of interpretability saliency maps, we used default parameters of the iNNvestigate implementation of Deep Taylor \cite{alber2019innvestigate}. 
For uncertainty estimation we used a total of $T=20$ dropout samples with dropout distributed across all layers \cite{BDNN}. 
During active learning the batch size for our experiments was set to $16$. % samples from each input of testing images (ref. Eq.\ref{alg1:topn} in Algorithm \ref{alg1}) following \cite{MahapatraMICCAI2018, BozorgtabarCVIU2019}. %In the results section we discuss further the interplay between the number of queried samples and the number of training iterations. %Implemented code is available at https://github.com/*****

\snm{As shown in Figure~\ref{fig:SSOrdinal} the encoder stage has 3 layers of $256,128,64$ neurons. The output is a $32$ dimensional latent feature vector which is fed to the decoding stage. The output is supposed to reconstruct the original input using the mean square error loss.}
